# Supplementary material for: Hierarchical Uncertainty Exploration via Feedforward Posterior Trees
Source: arXiv:2405.15719 source file (2024-05-24)
Supplement: Supplementary file 9 [file CelebA_colorization_figure_appendix.tex]

\begin{figure}[t]

{\input{texfigures/CelebA_colorization_appendix_subfig1}}

\vspace{0.1cm}
{\input{texfigures/CelebA_colorization_appendix_subfig4}}

\caption{\textbf{More CelebA-HQ colorization results.}}
\label{fig:app-more-celebahq-color}
\end{figure}
