# Supplementary material for: Hierarchical Uncertainty Exploration via Feedforward Posterior Trees
Source: arXiv:2405.15719 source file (2024-05-24)
Supplement: Supplementary file 15 [file CelebA_mouth_inpaint_appendix_subfig1.tex]

\begin{subfigure}{1cm}
    \centering
    $ \scriptstyle \text{GT}$\\
    \includegraphics[scale=0.12]{media/appendix/CelebA_mouth_inpaint1/img_gt.png}
\end{subfigure}
\begin{subfigure}{1cm}
    \centering
    $ \scriptstyle \text{Input}$\\
\includegraphics[scale=0.12]{media/appendix/CelebA_mouth_inpaint1/img_input.png}
\end{subfigure}

\vspace{-1.2cm}
\begin{nscenter}
\begin{forest}
  before typesetting nodes={
    for tree={
        font=\footnotesize,
      content/.wrap 2 pgfmath args={    {\footnotesize #2}\\\includegraphics[scale=0.12]{#1}}{content()}{title()},
    },
    where={isodd(n_children())}{calign=child, calign child/.wrap pgfmath arg={#1}{int((n_children()+1)/2)}}{},
  },
  forked edges,
  /tikz/every node/.append style={font=\footnotesize},
  for tree={
    parent anchor=children,
    child anchor=parent,
    align=center,
    l sep'= 1mm,
    s sep'= 2.5mm,
    fork sep'=0mm,
    inner sep = -2.5pt,
    edge={line width=0.5pt},
    font=\footnotesize,
  },
  [media/appendix/CelebA_mouth_inpaint1/Level_0/img_000.png, title={ {$ \scriptstyle \text{MMSE}$}}
    [media/appendix/CelebA_mouth_inpaint1/Level_1/img_000.png, title={ $\scriptstyle p=0.09$}
      [media/appendix/CelebA_mouth_inpaint1/Level_2/img_000.png, title={ $\scriptstyle p=0.02$}]
      [media/appendix/CelebA_mouth_inpaint1/Level_2/img_001.png, title={ $\scriptstyle p=0.07$}]
      [media/appendix/CelebA_mouth_inpaint1/Level_2/img_002.png, title={ $\scriptstyle p=0.01$}]
    ]
    [media/appendix/CelebA_mouth_inpaint1/Level_1/img_001.png, title={ $\scriptstyle p=0.50$}
      [media/appendix/CelebA_mouth_inpaint1/Level_2/img_003.png, title={ $\scriptstyle p=0.07$}]
      [media/appendix/CelebA_mouth_inpaint1/Level_2/img_004.png, title={ $ \scriptstyle p=0.15$}]
      [media/appendix/CelebA_mouth_inpaint1/Level_2/img_005.png, title={ $\scriptstyle p=0.29$}]
    ]
    [media/appendix/CelebA_mouth_inpaint1/Level_1/img_002.png, title={ $\scriptstyle p=0.40$}
      [media/appendix/CelebA_mouth_inpaint1/Level_2/img_006.png, title={{ $\scriptstyle p=0.14$}}]
      [media/appendix/CelebA_mouth_inpaint1/Level_2/img_007.png, title={$\scriptstyle p=0.17$}]
      [media/appendix/CelebA_mouth_inpaint1/Level_2/img_008.png, title={ $\scriptstyle p=0.10$}]
    ]
  ]
\end{forest}
\end{nscenter}
