# Supplementary material for: Hierarchical Uncertainty Exploration via Feedforward Posterior Trees
Source: arXiv:2405.15719 source file (2024-05-24)
Supplement: Supplementary file 18 [file CelebA_mouth_inpaint_figure_appendix.tex]

\begin{figure}[ht]

{\input{texfigures/CelebA_mouth_inpaint_appendix_subfig2}}

\vspace{0.1cm}
{\input{texfigures/CelebA_mouth_inpaint_appendix_subfig3}}

% \vspace{0.1cm}
% {\input{texfigures/CelebA_mouth_inpaint_appendix_subfig4}}

\caption{\textbf{More mouth inpainting results.}}
\label{fig:app-more-mouth-inpaint}
\end{figure}
